# Supplementary material for: Reinforcement Learning Control of Quantum Error Correction
Source: arXiv:2511.08493 source file (2026-06-19)
Supplement: Supplementary file 10 [file toc.tex]

\maketitle
\tableofcontents
